# Supplementary material for: Password Strength Signaling: A Counter-Intuitive Defense Against Password Cracking
Source: arXiv:2009.10060 source file (2021-08-16)
Supplement: Supplementary file 1 [file AppendixBITEOPT.tex]

\section*{Background: BITEOPT algorithm}\label{appendix:BITEOPT}

 In our experiments, we used BITmask Evolution OPTimization (BITEOPT) algorithm \cite{biteopt} to compute the quasi-optimal signaling matrix $\osm$.  Derivative-free optimization is active research area with many mature solvers with simple interface, e.g., CMA-ES \cite{Hansen06thecma}, NOMAD \cite{AuLeTr09a, NOMAD}, DAKOTA \cite{inbook}. BITEOPT is a free open-source stochastic non-linear bound-constrained derivative-free optimization method (heuristic or strategy). BiteOpt took 2nd place (1st by sum of ranks) in BBComp2018-1OBJ-expensive competition track \cite{BBComp}. 

BITEOPT maintains a population list of previously evaluated solutions that are ordered in cost (objective function value). The whole population evolves towards a lower cost. On every iteration, the solution with the highest cost in the list can be replaced with a new solution, and the list is reordered.  The solution vectors are spanned apart from each other to cover a larger parameter search space collectively. Besides that, a range of parameter randomization and the "step in the right direction" (Differential Evolution "mutation") operations are used that probabilistically make the population evolve to be ``fittest’’ ones (lower cost solutions). BITEOPT’s hyper-parameters (probabilities) were pre-selected and are not supposed to be changed.

One iteration of BITEOPT is in essence a state automate which includes 7 stages (see Fig. \ref{fig:biteopt} where  $q_1,\ldots,q_4$ are state transformation probability):
\begin{itemize}
\item Initialization stage: randomly generate a list of solutions $\mathbf{x}$ (population size is $size_p$) ordered in cost, chose one of 4 best solutions to be evolved, $x_{new}=x_{best}$. 
\item Stage 1: perform the ``step in the right direction’’ operation using the random previous solution, chosen best and worst solutions, plus a difference of two other random solutions. This is conceptually similar to Differential Evolution's ``mutation’’ operation. The used worst solution is randomly chosen from 3 worst solutions.
$$x_{new} = x_{best}-\frac{\left(x_{worst}-x_{rand}-(x_{rand2}-x_{rand3})\right)}{2}.$$
\item Intermediate stage.
\item Stage 2: perform ``bitmask inversion’’ operation for a single (or multiple) parameter value(s). Below, $i$ is either equal to $rand(1, d(d-1))$ or in the range $[1: d(d-1)]$, depending on a hyper-parameter $AllpProb$. $\gg$ is a bit shift-right operation, $MantSize$ is a constant equal to 54, $MantSizeSh$ is a hyper-parameter that limits bit shift operation range. Actual implementation is more complex as it uses average of two such operations.
$$mask = (2^{MantSize} - 1)\gg \lfloor rand(0\ldots1)^4\cdot MantSizeSh\rfloor,$$
$$x_{new}[i] = \frac{\lfloor x_{new}[i]\cdot2^{MantSize}\rfloor \otimes mask}{2^{MantSize}}.$$
\item Stage 3: perform the ``random move around’’ operation. This operation is performed twice.
$$ x_{new}[i]=x_{new}[i]-rand(-1\ldots1)\cdot q_3 \cdot (x_{new}[i])-x_{rand}[i].$$
\item Stage 4: An alternative randomization method is used involving the best solution, centroid vector and a random solution.
\begin{equation*}
\begin{aligned}
&x_{new}[i] = x_{new}[i]+{(-1)}^j(x_{cent}[i]-x_{new}[i]), \\ &i=1,\ldots,d(d-1), \;s\in1,2=\left(rand(0\ldots1)<0.5?1:2\right)
\end{aligned}
\end{equation*}
\item Stage 5: perform ``short-cut’’ parameter vector change operation.
$$z = x_{new}[rand(1\ldots d(d-1))],$$
$$x_{new}[i]=z, \;\forall i =1, \ldots, d(d-1).$$
\item Decision stage:  If the cost $x_{new}$ is less than the worst cost of current population, then $x_{new}$ is accepted; otherwise, it will be rejected.
\end{itemize}

\begin{figure}[ht]
\begin{center}
\begin{tikzpicture}[shorten >=1pt,node distance=1.8cm,on grid]
  \node[state,initial]   (init)                {Init};
  \node[state]             (inter) [above right=of init] {Inter};
  \node[state]		(q_1) [below right =of init] {1};
  \node[state] 		(q_2) [right = of inter] {2};
  \node[state]		(q_3)[right = of q_2] {3};
  \node[state] 		(q_4) [below = of q_2, yshift=0.5cm] {4};
  \node[state] 		(q_5) [right = of q_4] {5};
  \node[state,accepting] (deci) [right=of q_5] {Deci};
  \path[->] (init) edge	node [above] {$q_1$} (inter)
                  	edge		node [below] {} (q_1)
		(q_1)	 edge[bend right, below]	node[above] {$q_4$} (q_5)
			 edge[bend right, below]	node[below] {} (deci)
		(inter) edge	(q_2)
			 edge	node[above]{$q_2$}(q_4)
		(q_2) edge 	node[above]{$q_3$}(q_3)
		(q_2) edge 	node[below]{$q_4$}(q_5)
		(q_2)	 edge (deci)
		(q_4) edge	node[below]{$q_4$}(q_5)
			 edge[bend right, below] (deci)
		(q_3) edge	node[right]{$q_4$}(q_5)
			 edge (deci)
		(q_5) edge (deci)
       ;
\end{tikzpicture}
\caption{State automate of one iteration of BITEOPT}
\label{fig:biteopt}
\end{center}
\end{figure}
