# Supplementary material for: Password Strength Signaling: A Counter-Intuitive Defense Against Password Cracking
Source: arXiv:2009.10060 source file (2021-08-16)
Supplement: Supplementary file 2 [file appendix.tex]

\section{Labeling Passwords Strength}\label{appendix:labelstrength}
Based on how $score$ is defined password strength can be classified into the following catorgrioies.
\subsubsection{composition strength}
For many years, $score(pw)$ was a function of LUDS: counts of \textbf{l}ower-and  \textbf{u}ppercase letters, \textbf{d}igits and \textbf{s}ymbols. As a descendent of LUDS, NIST entropy, recommended by the agency in 2013~\cite{burr2011sp}, remains an influential metric for password strength.

\subsubsection{pattern strength}
\textsf{zxcvbn}~\cite{wheeler2016zxcvbn} combines common token lookup and pattern matching to heuristically estimate a guessing attack directly, Instead of estimating a virtual guessing attack, Probabilistic Context-Free Grammars (PCFGs)~\cite{SP:WAMG09,SP:KKMSVB12,NDSS:VerColTho14}, Markov Models~\cite{NDSS:CasDurPer12,Castelluccia2013,SP:MYLL14,USENIX:USBCCKKMMS15}, Neural Networks~\cite{USENIX:MUSKBCC16} build a checking dictionary to crack passwords. We consider strength calculated from these cracking models a form of pattern strength.

\subsubsection{frequency strength}
Composition strength and pattern strength both require plaintext password data to compute, while frequency strength only requires the frequency of each password in the dataset. This allows for the use of non-plaintext password databases e.g. of the type provided by~\cite{NDSS:BloDatBon16}. We adopt frequency strength in this work.

Given some password dataset $D, |D| = N$, and the frequencies for each password $f_i$ we can create a partition of the dataset with roughly equivalent size in descending order of password frequency. In particular, we divide the probability space $[0,1]$ evenly, i.e., setting strength thresholds to be $0, 1/d, 2/d, \ldots, d/d$. Given a frequency list $D_f$ and the frequency of a password $f_k$, if $i/d < \sum_{j = 1}^k f_j/N \le (i+1)/d$ for some $i\in 0, \ldots d-1$, we label password of frequency $f_k$ with strength level $i$.

Now we propose a heuristic algorithm to partition the password dataset as even as possible with respect to probability mass.
Suppose there are $d$ buckets representing $d$ strength levels, we label strength for password equivalence classes backward, handing the tough nut first. We maintain 4 variables: $probMass$ denoting the probability mass of current password equivalence class, $volume$ the probability mass that has been ``poured'' in the current bucket, $capacity$ the presumed ceiling of probability mass for the current bucket, $labeledProb$ the probability mass of passwords that have been labeled with a strength level.  Initially, $capacity$ of the last bucket is $1/d$, $volume$ of the last bucket is the probability of the last equivalence class $\frac{f_n}{N}*c_n$,  If $\frac{f_n}{N}*c_n\ge1/d$ which is typically the case, even though this is a violation of the constraint $volume\le capacity$, we still allow last equivalence class to be put in the last bucket (only for the first violation); If $\frac{f_n}{N}*c_n < 1/d$ we keep adding equivalence class until the bucket is full or just beginning to overflow. Then we move to the second to last bucket and  $capacity$ is updated as $(1-labeledProb)/(d-1)$. This process goes on until we have labeled all passwords in the frequency list. After the labeling,  the largest frequencies all for labels are output as the strength thresholds. Details can be found in Algorithm \ref{algo:criterion}. 

\begin{algorithm}
\caption{Label strength levels for passwords}
\label{algo:criterion}
\begin{algorithmic}[h1]
\REQUIRE{Equivalence class list $D_{eq} = \{(f_1, c_1),\ldots,(f_n,c_n)\}$, number of strength levels $d$}
\ENSURE{Strength thresholds $\{t_0,\ldots,t_{d-1}\}$}
\STATE $probMass = 0$
\STATE $volume = 0$
\STATE $labeledProb = 0$
\FOR{i=n \TO 1}
\STATE $probMass \leftarrow \frac{f_i}{N}\cdot c_i$
\STATE $volume += probMass$
\STATE $capacity = (1-labeledProb) /d$
    \IF{$volume > capacity$}     \COMMENT{only first violation of the constraint $volume \le capacity $ is allowed}
    \STATE set strength level of pwds with frequency $f_i$ to be $d-1$
    \STATE $labeledProb \mathrel{+}= volume$
    \STATE $volume = 0$
    \STATE $d \mathrel{-}= 1$
    \ELSE     \COMMENT{no violation}
    \STATE set strength level of pwds with frequency $f_i$ to be $d-1$\;
    \ENDIF
\ENDFOR
\RETURN $\{t_0,\ldots,t_{d-1}\}$, where $t_i$ is the largest frequency with label $i$.
\end{algorithmic}
\end{algorithm}

\section{Strength Oracle}\label{appendix:oracle}
Based on frequency thresholds and estimated frequency obtained from count sketch, we can construct a strength oracle.  
\begin{algorithm}[h]
\caption{Strength oracle $\mathsf{getStrength()}$}
\label{algo:strength}
\begin{algorithmic}[1]
\REQUIRE{$\mathcal{O}_f$, $pw_u$, $\{t_0,\ldots,t_{d-1}\}$}
\ENSURE{strength level of $pw_u$}
\STATE $\tilde{f}(pw_u) \leftarrow \mathcal{O}_f(pw_u)$
\FOR{$i=d-1$  \TO  0}
	\IF{$\tilde{f}(pw_u) <= t_i$}
		\RETURN $i$\;
	\ELSE
		\COMMENT{If the estimated frequency is larger than $t_0$, it will be considered as weak as level 0 pwds}
		\RETURN 0
	\ENDIF
\ENDFOR
\end{algorithmic}
\end{algorithm}
